# Supplementary material for: Optimal structured light waves generation in 3D volumes using communication mode optics
Source: arXiv:2411.10865 ancillary file (2025-05-14)
Supplement: Supplementary file 1 [file Supplement_1.pdf]

# Optimal structured light waves generation in 3D volumes using communication mode optics: supplemental document

## 1. SUPPLEMENTARY NOTE 1: SINGULAR VALUE DECOMPOSITION AND MAXIMIZATION PROPERTY OF THE COMMUNICATION MODES

The source  $\{|\Psi_{S,j}\rangle\}$  and receiving  $\{|\Phi_{R,j}\rangle\}$  eigenfunctions are computed from the eigen-equations associated with the operators  $G_{SR}^\dagger G_{SR}$  and  $G_{SR} G_{SR}^\dagger$ :

$$G_{SR}^\dagger G_{SR} |\Psi_{S,j}\rangle = |s_j|^2 |\Psi_{S,j}\rangle, \quad (\text{S1a})$$

$$G_{SR} G_{SR}^\dagger |\Phi_{R,j}\rangle = |s_j|^2 |\Phi_{R,j}\rangle, \quad (\text{S1b})$$

in which the eigenvalues  $|s_j|^2$ , the squared amplitude of the singular values  $s_j$  of  $G_{SR}$ , are the same for both operators. Additionally, the eigenfunctions satisfy the following one-to-one relation between their eigen-spaces [1]:

$$G_{SR} |\Psi_{S,j}\rangle = s_j |\Phi_{R,j}\rangle. \quad (\text{S2})$$

The relations established in Eq. (S1) are the core of the singular value decomposition (SVD) modal optics and its communication modes [1]. Each source eigenfunction  $|\Psi_{S,j}\rangle$  in the source space creates a resulting wave in the receiving space that has the form of the receiving eigenfunction  $|\Phi_{R,j}\rangle$  weighted by the complex amplitude  $s_j$ .

Assuming that the source and the receiving spaces contain a finite number of source and receiving points,  $N_S$  and  $N_R$ , rearranging Eq. (S2) by isolating the coupling operator  $G_{SR}$ , we obtain the expression for the SVD of  $G_{SR}$ :

$$G_{SR} = \sum_{j=1}^{N_m} s_j |\Phi_{R,j}\rangle \langle \Psi_{S,j}|, \quad (\text{S3})$$

in which  $N_m$  is the smaller of  $N_S$  and  $N_R$ . From  $N_m < j \leq N_{\text{large}}$ , in which  $N_{\text{large}}$  is the larger of  $N_S$  and  $N_R$ , the singular values  $s_j$  are identically zero [1]. In matrix form, Eq. (S3) can be written as:

$$G_{SR} = V D_{\text{diag}} U^\dagger, \quad (\text{S4})$$

where  $V$  is a  $N_R \times N_m$  matrix whose columns are the receiving eigenfunctions  $|\Phi_{R,j}\rangle$ , with  $1 \leq j \leq N_m$ ;  $D_{\text{diag}}$  is a diagonal  $N_m \times N_m$  matrix whose diagonal elements are the singular values  $s_j$ ; and  $U$  is a  $N_S \times N_m$  matrix whose columns are the source eigenfunctions  $|\Psi_{S,j}\rangle$ . Additionally, an important property that comes from Eq. (S4) is that the sum  $S$  of the coupling strengths  $|s_j|^2$  is finite and it can be obtained directly from the elements  $g_{ij}$  [Eq. (2) in the main text] of  $G_{SR}$ , without solving its SVD, as:

$$S = \sum_{q=1}^{N_m} |s_j|^2 = \sum_{i=1}^{N_R} \sum_{j=1}^{N_S} |g_{ij}|^2. \quad (\text{S5})$$

Eq. (S5) tells us that the number of communication modes and their coupling strengths are bounded for a given distribution of source and receiving points. Additionally, the source and receiving eigenfunctions computed from Eq. (S4) are also unique to a particular distribution of source and receiver points. Therefore it is not possible to obtain more orthogonal communication modes by performing linear combinations of these eigenfunctions. To increase the number of communication modes, we must modify the distribution of source and receiving points, leading to a new coupling operator matrix and thus to another SVD solution [1].

Now we derive the maximization properties of the communication mode pairs,  $\{|\Psi_{S,j}\rangle\}$  and  $\{|\Phi_{R,j}\rangle\}$ , computed from the eigen-equations of Eq. (S1). Our derivation follows the argument developed in Ref. [2] and it is based on finding which normalized source function  $\Psi_n(\mathbf{r}_S)$  (here the index  $n$  means normalized) gives raise to a resulting wave  $\phi(\mathbf{r}_R)$  in the receiving space with the largest possible magnitude  $|g|^2$ , here defined as:

$$|g|^2 = \int_{V_R} \phi^*(\mathbf{r}_R) \phi(\mathbf{r}_R) d^3 \mathbf{r}_R, \quad (\text{S6})$$

in which  $V_R$  stands for a finite volume containing the receiving space.

We start by recalling that the resulting wave  $\phi(\mathbf{r}_R)$  associated with a source function  $\Psi_n(\mathbf{r}_S)$  is given by:

$$\phi(\mathbf{r}) = \int_{V_S} G_{RS}(\mathbf{r}, \mathbf{r}_S) \Psi_n(\mathbf{r}_S) d^3 \mathbf{r}_S, \quad (\text{S7})$$

for a finite volume  $V_S$  containing the source space. Notice that Eq. (S7) is the integral form of Eq. (4) in the main text. Instead of a collection of source points, here we are assuming a continuous source function. Provided that our source points are close enough to each other, satisfying the criteria discussed in Supplementary Note 3, our derivation, based on continuous source and receiving functions, also applies for a collection of source and receiving points, analyzed in the main text. In view of that, substituting Eq. (S7) into Eq. (S6) yields:

$$|g|^2 = \int_{V_S} \Psi_n^*(\mathbf{r}'_S) \int_{V_S} K(\mathbf{r}'_S, \mathbf{r}_S) \Psi_n(\mathbf{r}_S) d^3 \mathbf{r}'_S d^3 \mathbf{r}_S, \quad (\text{S8})$$

in which we defined the kernel  $K(\mathbf{r}'_S, \mathbf{r}_S)$  as:

$$K(\mathbf{r}'_S, \mathbf{r}_S) = \int_{V_R} G_{RS}^*(\mathbf{r}_R, \mathbf{r}'_S) G_{RS}(\mathbf{r}_R, \mathbf{r}_S) d^3 \mathbf{r}_R, \quad (\text{S9})$$

which constitutes an Hermitian operator since  $K(\mathbf{r}'_S, \mathbf{r}_S) = K^*(\mathbf{r}_S, \mathbf{r}'_S)$ . Additionally, this kernel satisfies the following property:

$$\int_{V_S} \int_{V_S} |K(\mathbf{r}'_S, \mathbf{r}_S)|^2 d^3 \mathbf{r}'_S d^3 \mathbf{r}_S < \infty, \quad (\text{S10})$$

as both the source and receiving spaces are assumed to be defined over finite volumes,  $V_S$  and  $V_R$ , and the kernel  $K(\mathbf{r}'_S, \mathbf{r}_S)$  is a continuous bounded function. Notice that we are assuming that the source and receiving spaces are completely separated from each other, with no overlapping between them, as illustrated from the distribution examples in Figs 1(b-d) in the main text. Consequently,  $K(\mathbf{r}'_S, \mathbf{r}_S)$  does not present any singularities as the term  $|\mathbf{r}_R - \mathbf{r}_S|$  in the expression of  $G_{RS}$  [see Eq. (1) in the main text] always yields non-zero values. Therefore, with Eq. (S10) holding true, it allows us to conclude that the kernel  $K(\mathbf{r}'_S, \mathbf{r}_S)$  constitutes a Hilbert-Schmidt operator [1]. Since all Hilbert-Schmidt operators are compact,  $K(\mathbf{r}'_S, \mathbf{r}_S)$  is a compact Hermitian operator and thus its eigenfunctions form a complete set in the source space and their eigenvalues are real numbers. These results are formally proved by functional analysis. See Ref. [1] for deeper discussion, and also Ref. [3] for an introduction to the necessary results from functional analysis. The compactness also allows us to conclude that, with a sufficiently dense set of points in the source and receiving spaces, the resulting point-wise source and receiver eigenfunctions from the matrix problem converge to the solutions of the continuous problem.

Multiplying both sides of Eq. (S8) by  $\Psi_n(\mathbf{r}'_S)$  results in:

$$|g|^2 \Psi_n(\mathbf{r}'_S) = \int_{V_S} K(\mathbf{r}'_S, \mathbf{r}_S) \Psi_n(\mathbf{r}_S) d^3 \mathbf{r}_S, \quad (\text{S11})$$

where we have made use of our assumption that we are dealing with a normalized source function, i.e.,  $\int_{V_S} |\Psi_n(\mathbf{r}_S)|^2 d^3 \mathbf{r}_S = 1$ . It can be shown that the solutions of the integral equation in Eq. (S11) for the largest possible values of  $|g|^2$  are given when we choose  $\Psi_n(\mathbf{r}_S)$  as the normalized eigenfunctions of the kernel  $K(\mathbf{r}'_S, \mathbf{r}_S)$  [4]. In fact, these eigenfunctions correspond to the normalized versions of our source eigenfunctions  $\{|\Psi_{n,S,j}\rangle\}$  and the largest successive values of  $|g|^2$  correspond to our eigenvalues  $|s_j|^2$ .

Therefore, by ordering our source eigenfunctions  $\{|\Psi_{S,j}\rangle\}$  by decreasing size of their corresponding eigenvalues  $|s_j|^2$  we notice that: the source function  $|\Psi_{S,1}\rangle$  leads to the largest possible

magnitude of wave vector in the receiving space and this wave vector has the form of the receiving function  $|\Phi_{R,1}\rangle$ . Similarly,  $|\Psi_{S,2}\rangle$  leads to the second largest possible magnitude of wave vector in the receiving space having the form of  $|\Phi_{R,2}\rangle$ . We can proceed in a similar fashion for all the other source eigenfunctions. Thus, we can conclude that our communication mode pairs,  $\{|\Psi_{S,j}\rangle\}$  and  $\{|\Phi_{R,j}\rangle\}$ , are indeed the optimal modes that connect the source and receiving spaces in terms of magnitude of inner product. See Ref. [1] for an extended discussion of the properties of these operators and sets of eigenfunctions, and the SVD generally.

## 2. SUPPLEMENTARY NOTE 2: REQUIRED SOURCE FUNCTION FOR A GIVEN TARGET LIGHT DISTRIBUTION

Let  $|\Phi_T\rangle$  be our target profile in the receiving space  $H_R$ . In this space,  $|\Phi_T\rangle$  can be written as a linear superposition of the receiving eigenfunctions  $|\Phi_{R,j}\rangle$  as follows:

$$|\Phi_T\rangle = \sum_j a_j |\Phi_{R,j}\rangle, \quad (\text{S12})$$

in which the coefficients  $a_j$  are computed from the inner product between the target profile and the receiving eigenfunctions  $a_j = \langle \Phi_{R,j} | \Phi_T \rangle$ . Using the relation of Eq. (S2), we can determine the component of the source function that creates each component  $a_j |\Phi_{R,j}\rangle$  of the target profile:

$$G_{RS}(a_j |\Psi_{S,j}\rangle) = s_j(a_j |\Phi_{R,j}\rangle) \rightarrow G_{RS}\left(\frac{a_j}{s_j} |\Psi_{S,j}\rangle\right) = a_j |\Phi_{R,j}\rangle. \quad (\text{S13})$$

Therefore, summing up all these weighted source eigenfunctions  $(a_j/s_j) |\Psi_{S,j}\rangle$ , we obtain the required source function  $|\Psi_T\rangle$  in the source space  $H_S$  that creates the target profile  $|\Phi_T\rangle$  in the receiving space [1]:

$$|\Psi_T\rangle = \sum_j \frac{a_j}{s_j} |\Psi_{S,j}\rangle = \sum_j \frac{1}{s_j} \langle \Phi_{R,j} | \Phi_T \rangle |\Psi_{S,j}\rangle, \quad (\text{S14})$$

which corresponds to Eq. (3) in the main text.

### 3. SUPPLEMENTARY NOTE 3: MAXIMUM ALLOWED VALUE FOR THE DISTANCES BETWEEN THE SOURCE POINTS

The source points must be close enough to each other such that the collection of these points behaves similarly to a continuous source, i.e., a set of uniform source patches covering the entire source plane. In particular, we need to make sure that the resulting wave amplitude created by a point source  $(x_s, y_s)$  at a given receiving point  $(x_r, y_r, z_r)$  is approximately the same as the one created by a uniform source that surrounds that point source. To satisfy this condition, we consider two paths connecting a given receiving point, one from a corner of the patch and another one from the middle of the patch (where the source point is located), as illustrated in Fig. S1(a). The waves that leave these two points at the source aperture result in destructive interference at the receiving point if the difference between the two path lengths is half the wavelength. Therefore, it is reasonable to assume that if the difference between these paths is less than half a wavelength, there is no significant difference whether we consider a point source or a uniform source patch. From this condition, we derive an upper limit for the allowed values of the spacing distances between the source points  $d_x$  and  $d_y$ .

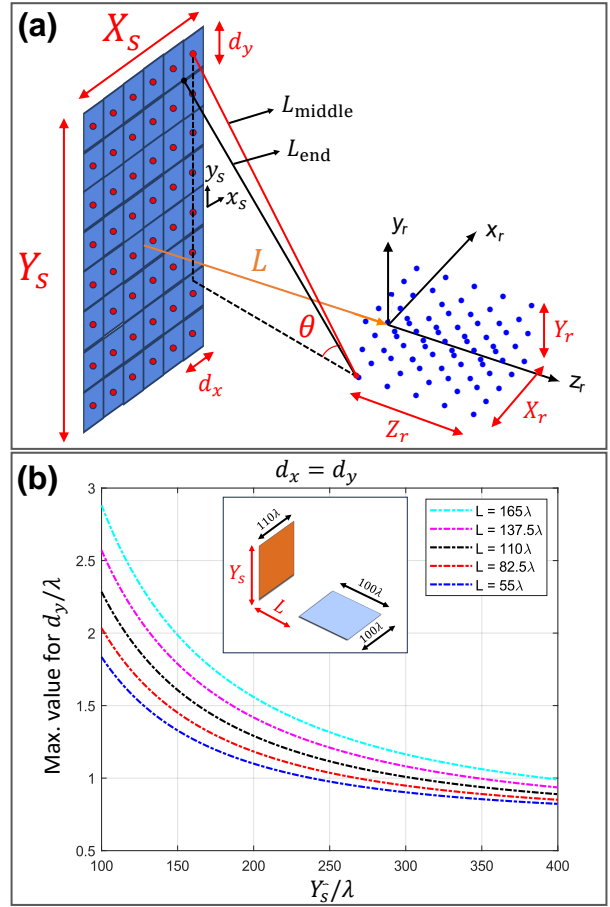

**Fig. S1. Estimating an upper limit value to the spacing distances between the source points. (a)** Schematic showing the array of source points spaced from each other by  $d_x$  and  $d_y$ . The collection of the source points (red dots) must behave essentially as a set of uniform source patches (blue squares) covering the entire source plane. For a given receiving point and source patch, we compute the difference between two path lengths: one connecting the middle of the patch  $L_{\text{middle}}$  (in red) and another one connecting one of the corners of the patch  $L_{\text{corner}}$  (in black). Setting this difference to be less than half a wavelength, we can assume that the resulting wave amplitude created by a point source (in the middle of the patch) at the receiving point is approximately equal to the one created by the patch. **(b)** Maximum allowed values for  $d_x = d_y$  for the source and receiving space of Fig. 1(b) - a single horizontal plane - as function of the number of source points along the  $y_s$  direction and for different values of the on-axis longitudinal separation distance  $L$  between the spaces.

Assuming that the spacing between the source points along the  $x_s$  and  $y_s$  directions are the same, i.e.,  $d_x = d_y$ , from Fig. S1(a), the difference between the two path lengths is:

$$|L_{\text{corner}} - L_{\text{middle}}| = \sqrt{2}(d_y/2) \sin \theta, \quad (\text{S15})$$

in which  $\theta$  is the angle subtended between the path with length  $L_{\text{middle}}$  and the horizontal plane where the receiving point is located, such that:

$$\sin \theta = \frac{y_s - y_r}{\sqrt{(x_s - x_r)^2 + (y_s - y_r)^2 + (L + z_r)^2}}. \quad (\text{S16})$$

The maximum difference  $|L_{\text{corner}} - L_{\text{middle}}|$  in Eq. (S15) between the two paths, that occurs for a maximum value for  $\theta$ ,  $\theta_{\text{max}}$ , is associated with a path connecting a source point at a corner of the source aperture to a receiving point at the opposite corner of the plane  $z_r = 0$ . For instance, a path connecting the point  $(x_s, y_s) = (X_s/2, Y_s/2)$  in the source plane to the point  $(x_r, y_r, z_r) = (-X_r/2, -Y_r/2, 0)$  in the receiving space, as depicted in Fig. S1(a). Therefore, setting the right side of Eq. (S15) to be smaller than  $\lambda/2$ , leads to the following condition for the spacing distances  $d_x$  and  $d_y$ :

$$d_x = d_y < \frac{2}{\sqrt{2}} \frac{\lambda/2}{\sin \theta_{\text{max}}} = \frac{2\lambda}{\sqrt{2}} \frac{\sqrt{(X_s + X_r)^2/4 + (Y_s + Y_r)^2/4 + L^2}}{Y_s + Y_r}. \quad (\text{S17})$$

For the source and receiving spaces of Fig. 1(a) of the main text, parameterized according to Table 1, in which we adopted  $d_x = d_y = \lambda$ , Eq. (S17) yields  $d_x = d_y < 1.20\lambda$ . If we increase the number of source points along the  $y_s$  direction to  $p_y = 311$  (resulting in  $Y_s = 310\lambda$ ), the criterion of Eq. (S17) yields  $d_x = d_y < 0.991\lambda$ , implying that the source points at the top and bottom  $y_s$  positions no longer behave as uniform source patches. To solve this issue, we must consider a denser array of source points ( $d_x = d_y < \lambda$ ) for those aperture regions. In Fig. S1(b) we show the maximum allowed value of  $d_y$  for different values of  $Y_s$  and  $L$ . Notice that as we move to source points located at higher  $y_s$  positions (i.e., away from the aperture center  $y_s = 0$ ), progressively lower values for the spacing distance  $d_x$  and  $d_y$  are demanded. Additionally, reducing the on-axis longitudinal separation distance  $L$  between the spaces also imposes lower values for these spacing distances.

For a set of receiving horizontal planes, such as the set of 10 uniformly spaced ones analyzed in Fig. 4 in the main text, the criterion of Eq. (S17) is more restrictive for the spacing distances  $d_x$  and  $d_y$  compared to a single horizontal since the transverse dimension of the receiving  $Y_r$  is no longer null. For the example shown in the main text and parameterized accordingly to Table 1, in which we adopted  $d_x = d_y = 0.5\lambda$ , Eq. (S17) yields  $d_x = d_y < 0.789\lambda$ .

#### 4. SUPPLEMENTARY NOTE 4: COUPLING STRENGTHS AND INTENSITY PROFILES OF COMMUNICATION MODES

##### A. Receiving points distributed in a horizontal plane

For this source-receiving-space configuration, the coupling strength curve is characterized by a series of steps. As we clarify below, the number of strongly coupled steps corresponds to the number  $N_z$  of effective longitudinal ( $z_r$  direction) modes supported by the configuration. Meanwhile, the number of modes within each step corresponds approximately to the number of effective transverse modes. There are essentially two types of transverse modes in each step: strongly coupled and partially coupled modes. There will also be weakly coupled transverse modes associated with wave tunneling escape [5], though these are so weak that they essentially do not show up in the main series of steps. The strongly coupled modes are those that couple strongly throughout the longitudinal length  $Z_r$  of the receiving space, and their coupling strengths correspond to the nearly flat region of the step. In contrast, partially coupled modes are modes that do not strongly couple all the way to the far end  $z_r = Z_r$  of the horizontal receiving plane, although they are able to couple relatively well at least into some fraction of the receiving space at the end closest to the source  $z_r = 0$ . These partially coupled modes give rise to the moderately steep fall-off in the coupling strength curve after the last strongly coupled mode on a given step. The number of strong effective transverse modes  $N_{x,\text{str}}$  and the number of effective longitudinal modes  $N_z$  can be computed as the maximum number of intensity fringes we can form in the receiving horizontal plane along its entire transverse  $X_r$  and longitudinal  $Z_r$  dimensions, respectively, as illustrated in Figs S2(a-b). For  $N_{x,\text{str}}$ , we compute the number of intensity fringes at the final longitudinal position ( $z_s = L + Z_r$ ) of the receiving space created by the two furthest source points along the source  $x_s$  transverse direction, i.e. with a spacing distance equal to the lateral extent  $X_s$  of the source plane. Since we can reasonably consider that  $X_s$  is significantly smaller than the longitudinal distance  $L + Z_r$ , we can use the one-dimensional paraxial heuristic number, defined in Ref. [1], which evaluates the number of effective modes in the case of transverse source and receiver lines. Thus, in our case,  $N_{x,\text{str}}$  is evaluated as:

$$N_{x,\text{str}} = \frac{X_r X_s}{(L + Z_r)\lambda}. \quad (\text{S18})$$

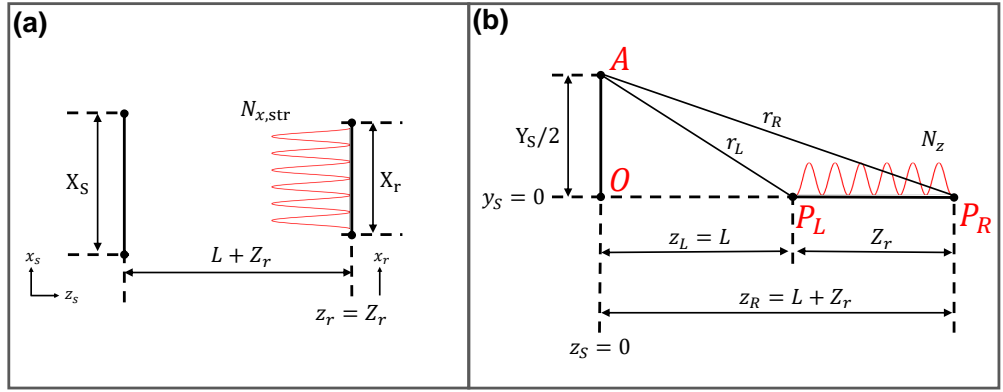

**Fig. S2. Number of effective modes in a transverse source plane and a horizontal receiving plane configuration.** (a) Schematic to determine the number of effective strong transverse modes  $N_{x,\text{str}}$  as the maximum number of intensity fringes we can form along the transverse width  $X_r$  of the receiving plane at the end of its longitudinal length ( $z_r = Z_r$ ). (b) Similarly, the number of effective longitudinal modes  $N_z$  is determined as the maximum number of intensity fringes we can form along the receiving longitudinal distance  $Z_r$ .

To evaluate the number  $N_z$  of effective longitudinal modes, we assume an off-axis source point at the vertical position  $y_s = Y_s/2$  and one at the origin  $y_s = 0$  [points A and O in Fig. S2 (b)] and compute the difference in path length between the waves from these points at the initial  $z_s = L$  and final  $z_s = L + Z_r$  longitudinal positions of the receiving plane [points  $P_L$  and  $P_R$  in Fig. S2(b)]. At point  $P_L$ , this difference is  $l_L = r_L - z_L = \sqrt{(Y_s/2)^2 + L^2} - L$  while at point  $P_R$ ,  $l_R = r_R - z_R = \sqrt{(Y_s/2)^2 + (L + Z_r)^2} - (L + Z_r)$ . Thus, as we proceed from point  $P_L$  to  $P_R$  we

pass through a number  $N_z$  of complete interference fringes along the  $z_r$  direction given by:

$$N_z = \frac{l_L - l_R}{\lambda} = \left( \sqrt{(Y_s/2)^2 + L^2} - \sqrt{(Y_s/2)^2 + (L + Z_r)^2} + Z_r \right) \frac{1}{\lambda}, \quad (\text{S19})$$

for any particular fixed phases of the point sources at A and O. If we imagine that we moved the off-axis source progressively from point O to point A, we could therefore progressively change the number of fringes  $N_z$ , and along the way, we could imagine that we could create approximately different fringe patterns, with different numbers of periods, that are orthogonal to one another. From Eq. (S19) we can also compute the vertical source distance  $Y_{n_z}$  required to generate a particular number  $n_z$  of longitudinal fringes. Replacing  $Y_s/2$  by  $Y_{n_z}$  and  $N_z$  by  $n_z$  in Eq. (S19) leads to:

$$Y_{n_z}/\lambda = \pm \frac{\sqrt{n_z[2(Z_r/\lambda) - n_z][4L(L + Z_r)/\lambda^2 + 2(Z_r/\lambda)n_z - n_z^2]}}{2[(Z_r/\lambda) - n_z]}. \quad (\text{S20})$$

In view of Eq. (S20), we can categorize the modes according to their behavior along the vertical source dimension, setting  $Y_{n_z}$  as a characteristic parameter. For the modes within the first step ( $n_z = 1$ ),  $Y_1$  corresponds to the extent in the  $y_s$  direction (relative to the center) of the intensity profiles of the source eigenfunctions. Meanwhile, for higher steps,  $1 < n_z \leq N_z$ ,  $Y_{n_z}$  corresponds to the vertical positions  $y_s = \pm Y_{n_z}$  where the source eigenfunction profiles are centered. To illustrate this, in Supplementary Video 1, we show the intensity profiles of all the first 250 well-coupled communication modes of the configuration parametrized as listed in Table 1. The coupling strengths of this configuration are shown in Fig. S3 (a), in which the vertical dashed lines highlight the last strong mode of each step and the inset sub-figure depicts the absolute values of  $Y_{n_z}$  computed from Eq. (S20). The strong modes of the first step correspond to the interval  $1 \leq j \leq 52$ , thus totaling a number of  $N_{x,\text{str}} = 52$  effective transverse modes, as predicted by Eq. (S18). Past these modes, we next find the partially coupled modes before we arrive at the strongly coupled modes of the near-flat region of the next step. In Fig. S3(b), we show the normalized intensity profiles of the last four strong modes ( $j = 49, \dots, 52$ ) and the first two partially coupled modes ( $j = 53, 54$ ) of the first step. As we move from one step to another, the source eigenfunction profiles progressively occupy higher vertical positions  $y_s = \pm Y_{n_z}$ , as predicted by Eq. (S20). As a result, their receiving eigenfunction profiles acquire an additional fringe along the  $z_r$  direction, thus providing progressively higher longitudinal spatial frequencies. This is illustrated in Fig. S3(c) in which we show the intensity profile of the last strong communication mode of the steps  $n_z = \{4, 8, 12, 14, 16, 18\}$ . Notice that as the vertical positions  $y_s = \pm Y_{n_z}$  approach the edges  $y_s = \pm Y_s/2$  of the source plane, more of the intensity profile of the source eigenfunction is compressed near these upper and lower edges of the finite source aperture. Associated with this compression, the receiving eigenfunction is no longer able to couple as strongly as the ones of the first steps throughout the entire length of the receiving space, as depicted in Fig. S3(d). For the purposes of discussion, we will still refer to these modes of the final steps as "strong" modes. Essentially, for these final steps, since their nominal values  $|Y_{n_z}|$ , given by Eq. (S20), approach the actual size of the source aperture ( $Y_s/2$ ), they are very close to passing the conventional diffraction limit for forming beams at the far end of the receiving space.

After the series of steps of up to  $n_z = 18$ , the singular values show a rapid fall-off decrease in their magnitude, as noted at the end of the coupling strength curve in Fig. S3(a) and also in Fig. S4 in which we show this coupling strength curve up to the first 1400 modes on a logarithmic scale. This ultimate rapid fall-off is a universal behavior in the analysis of communication modes, regardless of the shape of the receiving and source spaces [1]. Recently, this behavior has been explained as a consequence of the tunneling escape of waves from any arbitrary finite source volume [5]. By means of an analysis based on spherical waves, it has been shown that beyond a number of well-coupled modes, waves associated with subsequent modes must tunnel to escape the finite source volume. We expect that this transition from the propagating region to the tunneling escape region occurs precisely when the coupling strengths fall off rapidly. For our source-receiving configuration, the condition for the onset of tunneling escape of waves is essentially  $|Y_{n_z}| > Y_s/2$ , or equivalently,  $n_z > N_z$ . Figure S4 makes the clear point that, above some finite number of modes, the coupling strengths of subsequent modes drop rapidly, practically limiting the number of usable modes. As it has been argued in Ref. [5], this kind of fall-off is inevitable.

Equations (S18) and (S19) are useful to give us a sense of the total number of effective modes from the product  $N_{x,\text{str}} N_z$  before solving the SVD problem. This can only be a rough estimate

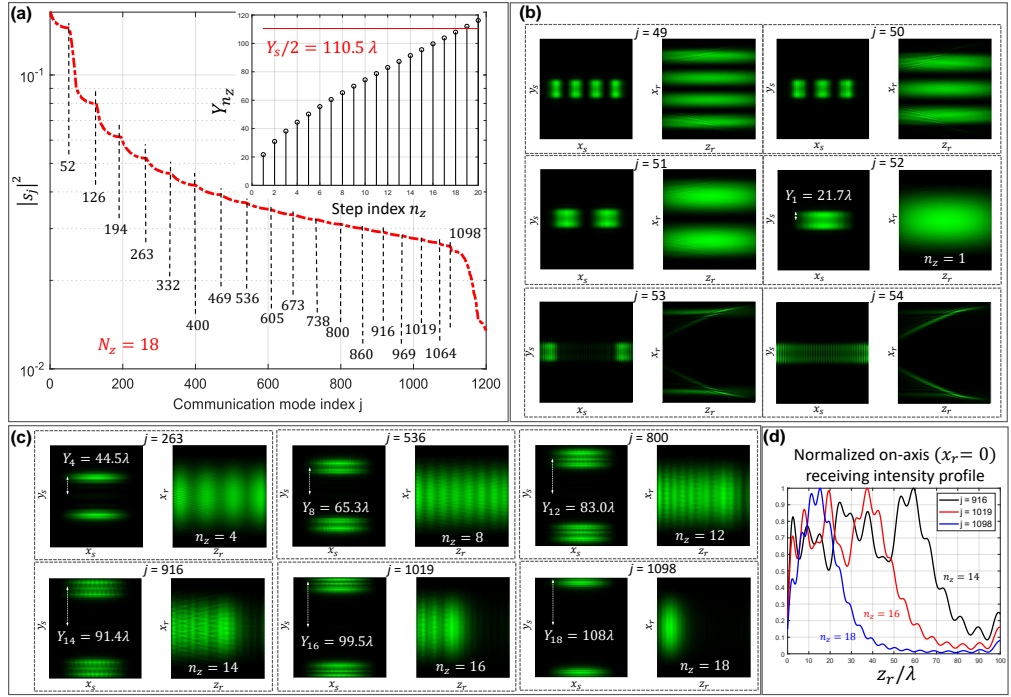

**Fig. S3. Communication modes and their coupling strengths associated with a transverse source plane and a horizontal receiving plane.** (a) Coupling strengths on a logarithmic scale and in order of decreasing size of their magnitude of the first 1200 modes for this configuration parameterized as listed on Table 1. The vertical dashed lines highlight the last strong mode of each step and the inset sub-figure depicts the characteristic vertical position  $Y_{n_z}$  of the source eigenfunctions of each step. Normalized amplitude of: (b) the last four strong modes and the first two partially coupled modes of the first step  $n_z = 1$ , (c) the last strong mode of the steps  $n_z = \{4, 8, 12, 14, 16, 18\}$ . (d) Normalized on-axis intensity profile along the receiving longitudinal distance for the last strong mode of the steps  $n_z = \{14, 16, 18\}$ .

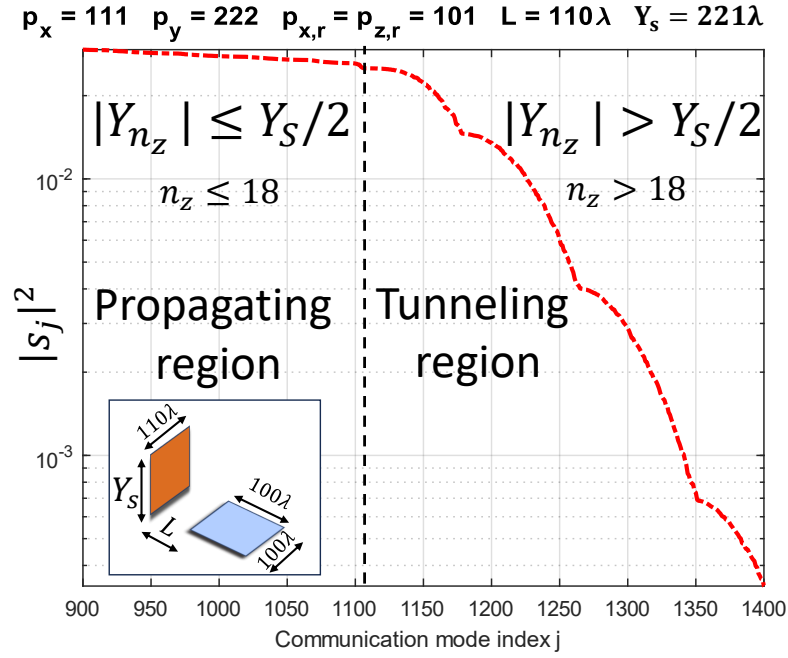

**Fig. S4.** Rapid fall-off decrease of the coupling strengths after the regions of well coupled modes (series of steps). Coupling strengths on a logarithmic scale of the source-receiving system configuration parameterized as listed on Table 1. The rapid fall-off of the coupling strengths is a consequence of the tunneling escape of waves from any arbitrary finite source volume. For the source-receiving-space configuration of a transverse plane and a horizontal receiving plane, the condition for the onset of tunneling escape of waves is when the vertical positions of the source eigenfunction profiles become larger than the source aperture size  $|Y_{n_z}| > Y_s/2$ .

because it does not count the partially coupled modes, particularly in the earlier steps, and in the later steps there may be not as many strongly coupled modes as in the first steps. This is illustrated in Fig. S5(a) which compares the coupling strengths for different values of the vertical dimension  $Y_s$  of the source plane and we highlight the indexes of the last strong mode of the blue curve (for  $Y_s = 166\lambda$ ). Furthermore, Fig. S5(a) clearly show that increasing the vertical dimension  $Y_s$  of the source substantially increases the number of useful modes.

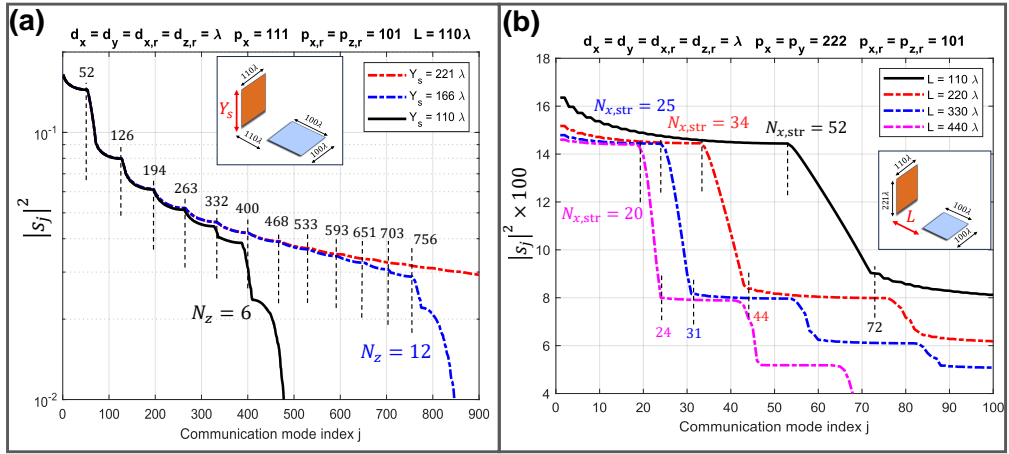

**Fig. S5. Influence of the finite source aperture vertical dimension  $Y_s$  and the longitudinal distance  $L$  on the number of strong modes.** Coupling strengths of the source-receiving system configuration parameterized as listed on Table 1 for (a) different values of  $Y_s$  (on a logarithmic scale) and (b) for different values of  $L$ . In (a) the dashed vertical lines highlight the last strong mode of each step of the blue curve ( $Y_s = 166\lambda$ ). In (b) these lines highlight the last strong mode of the first step and the first strong mode of the second step. Increasing the source vertical dimension  $Y_s$  increases the number of effective longitudinal modes  $N_z$ , i.e., the number of steps in the coupling strength curve. Meanwhile, decreasing the longitudinal distances between the spaces also promotes an increase of the number of strong transverse modes and partially coupled modes in each step.

The number of strong transverse modes  $N_{x, \text{str}}$  in each step can be controlled by changing the longitudinal distance  $L$ . This is shown in Fig. S5(b) which depicts the coupling strengths for different values of  $L$ . The upper vertical dashed lines highlight the last strong mode of the first step while the bottom lines highlight the first strong mode of the second step. As we move far from the paraxial limit, that is, by decreasing the longitudinal distance  $L$ , not only the number of strong transverse modes  $N_{x, \text{str}}$  increases but also the number of partially coupled modes  $N_{x, \text{part}}$ . In fact, for lower values of  $L$  we can even find partially strong modes from a previous step inside the region of strong modes of the next step. This is the case for  $L = 110\lambda$  (black curve) in which although the modes  $j = \{74, 79, 90, 92\}$  have coupling strengths smaller than that of the first strong mode of the second step ( $j = 72$ ), they are partially coupled modes of the first step (see Supplementary Video 1). Finally, as we approach the paraxial limit, we expect the number of partially coupled modes to follow:

$$N_{x, \text{part}} = \frac{X_r X_s}{L\lambda} - \frac{X_r X_s}{(L + Z_r)\lambda} = \frac{X_r X_s}{L\lambda} - N_{x, \text{str}}, \quad (\text{S21})$$

i.e., being evaluated as the difference between the number of intensity fringes at the near-longitudinal position of the receiving plane ( $z_r = 0$ ) and that at the end longitudinal position ( $z_r = Z_r$ ). For  $L = 440\lambda = 4X_s$  (magenta curve), Eq.( S21) yields  $N_{x, \text{part}} = 4$  which approaches the actual number of 3 partially coupled modes seen in this curve before its second step.

## B. Receiving space composed of a set of horizontal planes

The communication modes associated with this receiving space are closely related to the modes of a single horizontal plane. The substantial difference is that the additional degree of freedom afforded by the transverse direction  $y_r$  of the receiving space results in an increase in the number of modes. These additional modes have similar intensity profiles within all horizontal planes but with distinct amplitude profiles along the  $y_r$  direction. In Fig. S6(a), we show the coupling strengths  $|s_j|^2$  of the first 3500 modes, ordered by decreasing size of their magnitude, associated

with the source and receiving configuration of Fig. 1(c) in the main text with the values of the parameters listed in Table 1. The normalized squared amplitude of the source and receiving eigenfunctions of the first 250 well-coupled modes are shown in Supplementary Video 2. We notice that we can identify groups of communication modes whose receiving eigenfunctions are characterized by the same intensity profile over all horizontal planes but modulated by distinct amplitude profiles along the  $y_r$  direction. To illustrate this phenomenon, in Fig. S6(b), we zoom-in the region of the coupling strength curve containing the first 70 well-coupled modes. From this figure, we identify groups of modes (highlighted by circles), each of which contains 16 modes. The modes of the first group ( $j = 1, \dots, 16$ ) have the same 'V' shaped intensity profile over the horizontal planes but with this profile modulated by distinct amplitudes along the  $y_r$  direction, as seen from the sub-figures of Fig. S6(c). Each sub-figure shows the source (on the left) and the receiving (on the right) eigenfunction intensity profiles of some of the modes within the first group ( $j = \{1, 3, 5, 7, 9, 16\}$ ). The other modes within this group are degenerate modes of these ones. Notice incidentally that the 'V' shaped intensity profiles of these modes are similar to the first mode  $j = 1$  associated with a single horizontal plane of receiving points shown in Fig. 2(c) in the main text. In fact, this similarity also applies to the other groups of modes. To illustrate this, the last two sub-figures of Fig. S6 show the source and receiving intensity profiles associated with the first mode of the second and third groups ( $j = 17$  and  $j = 33$ ). Notice that the intensity profiles of these modes over the horizontal planes are similar to the third  $j = 3$  and fifth  $j = 5$  modes for a single horizontal receiving plane, shown in Fig. 2(c) in the main text.

### C. Cylinder surface as a receiving space

In contrast to the communication modes for a receiving horizontal plane in which the source eigenfunctions are symmetric with respect to the  $y_s = 0$  axis, the source eigenfunctions associated with a cylindrical receiving surface either present rotational symmetries when their intensity profiles are rotated for some angles with respect to the optical axis, or we can find pairs of eigenfunctions that are related to each other by a rotation angle. In Fig. S7(a) we show the coupling strengths  $|s_j|^2$  of the first 1000 modes, ordered by decreasing the size of their magnitude, associated with the source and receiving configuration of Fig. 1(d) in the main text with the values of the parameters listed in Table 1. The normalized intensity profiles of the first two communication modes are shown in Fig. S7(b). Their source eigenfunctions, shown on the left of each sub-figure, are related to each other by a rotation of  $180^\circ$ . Incidentally, this symmetry also applies to their receiving eigenfunctions whose intensity profiles are shown in the receiving surface [in which  $\phi_r = \text{atan}(y_r/x_r)$  is the azimuth coordinate of the receiving rings] and at the mid transverse plane  $z_r = Z_r/2$  of the receiving space (plots on the middle and on the right in each sub-figure). Finally, similarly to the previous distributions, as we progressively move to modes with less coupling strength, their receiving eigenfunctions acquire progressively higher longitudinal spatial frequencies. This is depicted in Fig. S7(c) which shows the intensity profile of communication modes from different regions of the coupling strength curve of Fig. S7(a) as highlighted by the arrows. In particular, the intensity profile of their receiving eigenfunctions consists of four straight spots extending along the entire receiving longitudinal distance and angularly spaced  $90^\circ$  from each other. The difference between these profiles is that they gradually acquire a large number of regions of maximum intensity along the longitudinal  $z_r$  direction. The intensity profiles of all the first 100 well-coupled communication modes are shown in Supplementary Video 3.

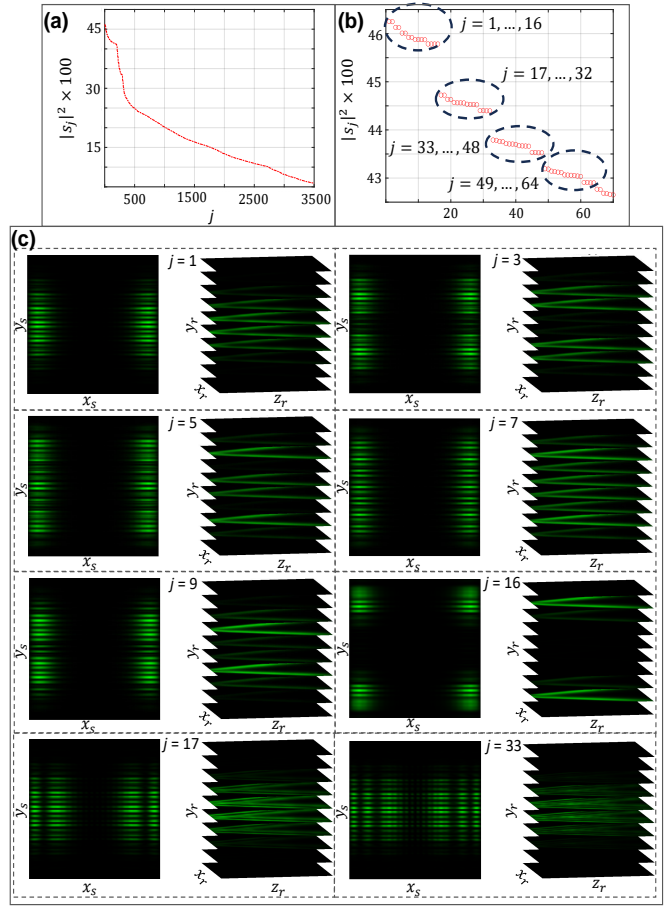

**Fig. S6. Communication modes and their coupling strengths associated with a transverse source plane and a set of uniformly spaced horizontal receiving planes.** (a) Coupling strengths  $|s_j|^2$  of the first 3500 communication modes, ordered by decreasing size of their magnitude, associated with the configuration of Fig. 1(c), parameterized as listed on Table 1. (b) A zoom-in visualization of the coupling strengths of the first 70 well-coupled modes. Each highlighted group of modes is characterized by having their receiving eigenfunctions built from the same intensity profile over the  $x_r z_r$  plane but modulated by distinct amplitude profiles along the  $y_r$  direction. (c) Normalized intensity profile of the source (on the left of each sub-figure) and receiving (on the right of each sub-figure) eigenfunctions of the communication modes  $j = \{1, 3, 5, 7, 9, 16\}$ , which belongs to the first highlighted group of modes. The other modes within this first group are degenerate modes of these ones. The two last sub-figures show the source and eigenfunctions of the first mode of the two subsequent groups ( $j = 17$  and  $j = 33$ ).

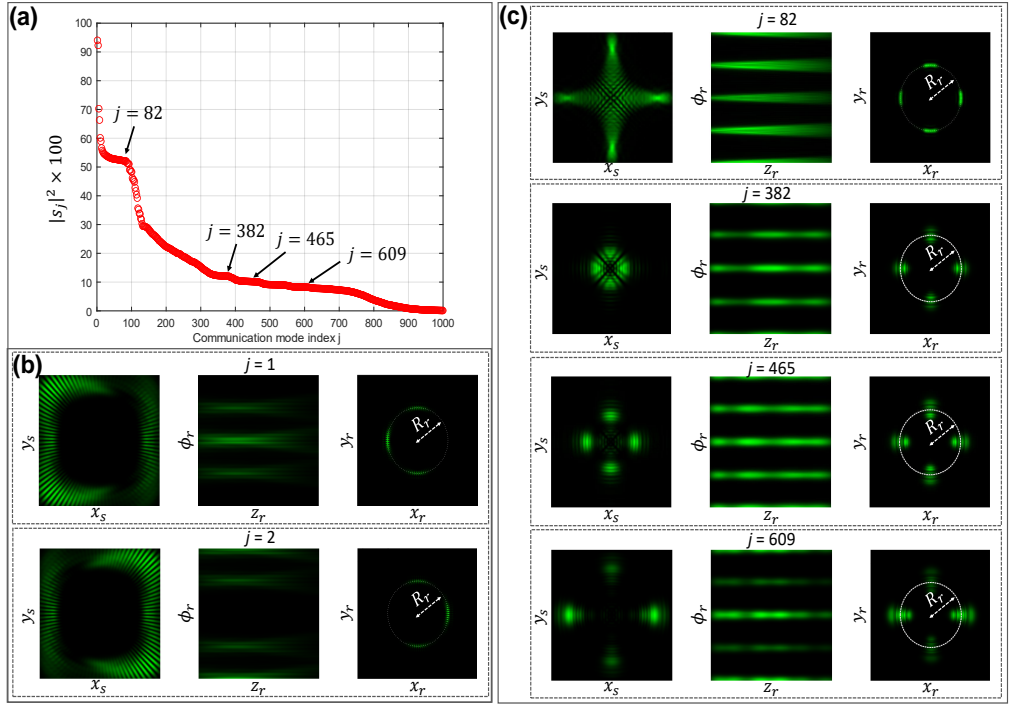

**Fig. S7.** Communication modes and their coupling strengths associated with a transverse source plane and a curved receiving space in which the receiving points are arranged over the longitudinal surface of a cylinder. (a) Coupling strengths in order of decreasing size of their magnitude of the first 1000 modes for this source-receiving system configuration parameterized as listed in Table 1. (b-c) Normalized intensity profiles of first two communication modes and of the modes highlighted by the arrows in (a). From left to right in each sub-figure: source eigenfunction in the source plane, receiving eigenfunction over the lateral cylindrical surface in terms of its azimuth angle and the longitudinal coordinate  $z_r$ , and at the mid transverse plane of the receiving space ( $z_r = Z_r/2$ ). In all the sub-figures,  $R_r$  refers to the radius of the cylindrical surface.

## 5. SUPPLEMENTARY NOTE 5: CHARACTERISTIC MINIMUM LONGITUDINAL LENGTH OF WAVE FIELD GENERATED BY A FINITE SOURCE TRANSVERSE PLANE

In this section, we derive the characteristic minimum length of wave field  $\Delta z$  our transverse source plane can create along the propagation direction at a particular receiving point  $P_0$  located at  $(x_r, y_r, z_r) = (x_{r,0}, y_{r,0}, z_{r,0})$ . This point  $P_0$  is located at a longitudinal distance  $z_s = z_0 = L + z_{r,0}$  from the source plane origin, as illustrated in Fig. S8(a). Additionally, assume that  $\Delta Y$  is the extent of the source intensity profile from the position  $y_s = y_{r,0}$ , connecting a source point that is aligned with the receiving plane (point O) to the furthest triggered source point located at point A in the source plane. Our derivation is based on the assumption that the waves created by these two source points interfere constructively at the point  $P_0$ , resulting in a maximum intensity at this point. At the same time, these waves interfere destructively at points  $P_L$  and  $P_R$  located on either side of  $P_0$  as shown in Fig. S8(a). Therefore, an estimation of the minimum length of wave field  $\Delta z$  our source aperture is able to create at position  $z_0$  corresponds to the separation distance between the points  $P_L$  and  $P_R$ :

$$\Delta z = (z_0 - z_L) + (z_R - z_0) = \Delta z_L + \Delta z_R. \quad (\text{S22})$$

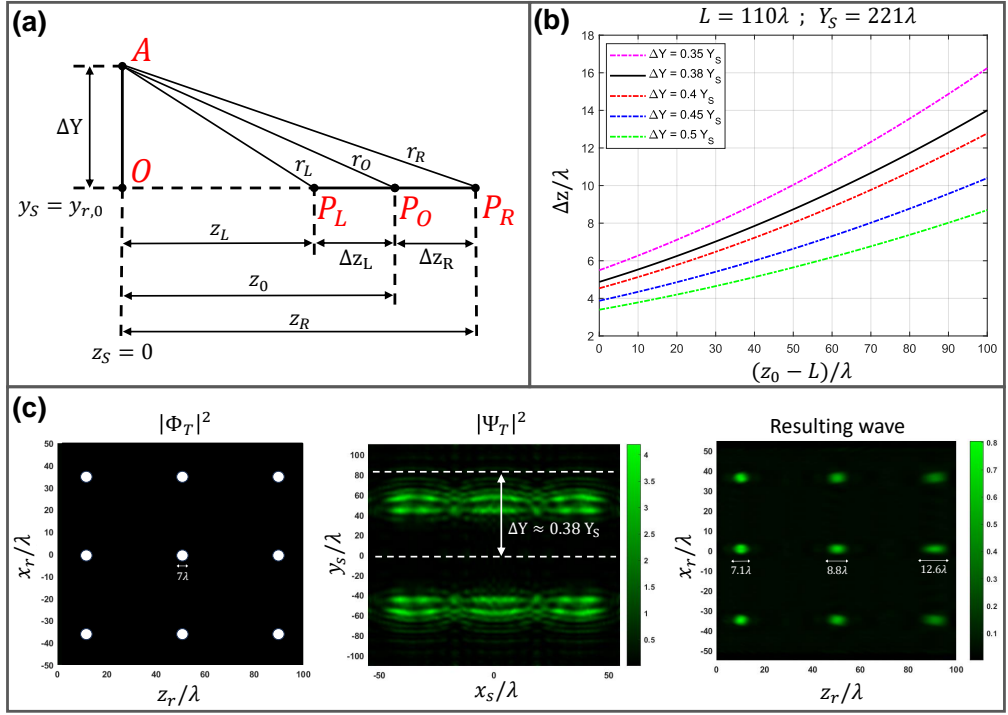

**Fig. S8.** Estimating the characteristic minimum length of wave field our finite transverse source aperture can create along the propagation direction. (a) Schematic in which a point  $P_0$ , for which we estimate characteristic minimum length of wave field, is located at a position  $z_s = z_0$  from the source aperture and at a receiving horizontal plane with  $y_r = y_{r,0}$ . We assume that the source field extends for a distance  $\Delta Y$  from the  $y_s = y_{r,0}$  plane, from a point O to a point A. The minimum length of wave field  $\Delta z = \Delta z_L + \Delta z_R$  is assigned as the distance between points  $P_L$  and  $P_R$  located on either side of  $P_0$  and is computed by presuming that the waves coming from points A and O interfere constructively at the point  $P_0$  while they interfere destructively at the points  $P_L$  and  $P_R$ . (b) Values of  $\Delta z$  as function of the receiving plane  $z$  position and for distinct  $\Delta Y$  values. We assume the source and receiving space configuration shown in Fig. 1(b) and parameterized as listed on Table 1, i.e., a single horizontal plane with  $y_{r,0} = 0$ . (c) A simulation example involving the reconstruction of a target profile that consists of  $7\lambda$  diameter circles placed at distinct longitudinal positions along the receiving plane. We are only able to resolve the circles located at  $z_r = 10\lambda$  (the ones close to the source plane), as  $\Delta z < 7\lambda$  at this position and  $\Delta z > 7\lambda$  at the other  $z_r$  positions ( $z_r = 50\lambda$  and  $z_r = 90\lambda$ ).

At the points  $P_L$  and  $P_R$  we must have a half a wavelength ( $\lambda/2$ ) difference for the relative path length between the waves from point O and from point A compared to that at point  $P_0$ . Since the distances from point A to all the three points  $P_0$ ,  $P_L$  and  $P_R$  are given by:

$$r_0 = \sqrt{(z_0)^2 + (\Delta Y)^2}, \quad (\text{S23a})$$

$$r_L = \sqrt{(z_0 - \Delta z_L)^2 + (\Delta Y)^2}, \quad (\text{S23b})$$

$$r_R = \sqrt{(z_0 + \Delta z_R)^2 + (\Delta Y)^2}, \quad (\text{S23c})$$

and the distances from point  $O$  to these points are respectively  $z_0$ ,  $z_L = z_0 - \Delta z_L$  and  $z_R = z_0 + \Delta z_R$ , computing the relative path lengths for each of the points  $P_L$  and  $P_R$  with respect to that of point  $P_0$  leads to:

$$\Delta s_L = (r_L - z_L) - (r_0 - z_0) = r_L - r_0 + \Delta z_L, \quad (\text{S24a})$$

$$\Delta s_R = (r_0 - z_0) - (r_R - z_R) = r_0 - r_R + \Delta z_R. \quad (\text{S24b})$$

Thus, setting  $\Delta s_L = \Delta s_R = \lambda/2$ , we find a set of two equations, one for  $\Delta z_L$  and another one for  $\Delta z_R$ :

$$\sqrt{(z_0 - \Delta z_L)^2 + (\Delta Y)^2} - \sqrt{(z_0)^2 + (\Delta Y)^2} + \Delta z_L = \lambda/2, \quad (\text{S25a})$$

$$\sqrt{(z_0)^2 + (\Delta Y)^2} - \sqrt{(z_0 + \Delta z_R)^2 + (\Delta Y)^2} + \Delta z_R = \lambda/2, \quad (\text{S25b})$$

which can be solved graphically or numerically for given values of  $z_0$  and  $\Delta Y$ . By solving for  $\Delta z_L$  and  $\Delta z_R$  from Eqs S25 (a-b), we sum these contributions up to compute the characteristic minimum length of wave field  $\Delta z$ , as in Eq. (S22). Values of  $\Delta z$  are shown in Fig. S8(b) as function of  $z_0$  and for distinct values of  $\Delta Y$ . Here we consider the source and receiving configuration shown in Fig. 2(a) in the main text, i.e., a single horizontal receiving space located at  $y_{r,0} = 0$ , in which the on-axis separation between the spaces is  $L = 110\lambda$  and the source plane has a total dimension of  $Y_s = 221\lambda$  along the  $y_s$  axis. Notice that  $\Delta z$  grows up quite rapidly with the distance  $z_r = z_0 - L$  within the receiving plane. Additionally, the extent  $\Delta Y$  of the source function is responsible not only for decreasing  $\Delta z$  but also its rate of change along the  $z$  direction. In Fig. S8(c) we provide a simulation example to demonstrate the fundamental limits imposed by our finite source aperture when we try to structure a spot with a longitudinal dimension smaller than  $\Delta z$ . Using the first  $M = 1200$  modes associated with the source and receiving configuration of Fig. 2(a) in the main text, we compute the required source function intensity  $|\Psi_T|^2$  and the resulting wave intensity at the horizontal receiving plane for a target profile consisting of  $7\lambda$  diameter circles centered at the following longitudinal positions along the receiving plane:  $z_r = 10\lambda$ ,  $z_r = 50\lambda$  and  $z_r = 90\lambda$ . While we are able to generate the circles located at  $z_r = 10\lambda$  relatively well, the resulting wave at the other circles' locations is characterized by spots with larger longitudinal dimensions, indicating that the values of the characteristic minimum length of wave field  $\Delta z$  at these locations are higher than the  $7\lambda$  longitudinal dimension of the target circles. In fact, their dimensions approximately satisfy the values of  $\Delta z$  given by the solid black curve of Fig. S8(b), computed for  $\Delta Y = 0.38Y_s$ , a value that matches with the extent of the source function intensity as depicted in Fig. S8(c).

For a receiving space that contains a set of parallel horizontal planes, a distinct maximum extent  $\Delta Y$  can be assigned to each horizontal plane  $y_r = y_{r,0}$  to compute the characteristic minimum length of wave field  $\Delta z$  at a certain longitudinal position  $z_r$  within each plane. Specifically, inner receiving planes can acquire higher values of  $\Delta Y$  compared to outer ones, as the maximum value we can assign to this parameter is  $\Delta Y = Y_s/2 - y_{r,0}$ . For this reason, it is expected that structuring small features at the outermost receiving planes is more challenging than at the inner ones. To illustrate this phenomenon, consider the receiving plane in which we projected the last ellipsoid slice (layer 8 in Fig. S11 located at  $y_{r,0} = 52.5\lambda$ ). Assuming  $\Delta Y = Y_s/2 - y_{r,0} = 75\lambda - 52.5\lambda = 22.5\lambda$ , i.e., the maximum value we can assign to this parameter for this plane, leads to  $\Delta z = 24.26\lambda$  at the center of that receiving plane ( $z_r = Z_r/2 = 25\lambda$ ). Because of this high value of  $\Delta z$  we are not able to completely resolve the last ellipsoid slice whose circle diameter is  $10\lambda$ .

## 6. SUPPLEMENTARY NOTE 6: INCORPORATION OF A PLANE WAVE PHASE FORM TO GENERATE THE TARGET AMPLITUDE PROFILES USING ONLY STRONGLY COUPLED COMMUNICATION MODES

From the analysis of the characteristic minimum longitudinal length of wave  $\Delta z$  provided in Supplementary Note 5, we notice the importance of having a source function profile  $|\Psi_T|^2$  with as large an extent  $\Delta Y$  as possible to properly resolve a given target intensity profile along all the longitudinal distances  $z_r$  of the receiving space. To increase  $\Delta Y$  we must modulate the target profile with a phase front of the form  $\exp(iQz_r)$ , in which  $0 \leq Q \leq k = 2\pi/\lambda$ . In Fig. S9 we demonstrate how this phase front affects the source function profile and its corresponding resulting wave in the receiving space for different values of  $Q$ . As noticed, as we progressively decrease  $Q$ , more of the target profile content  $|a_j|$  falls onto the range of well-coupled modes ( $j \leq 1200$ ) of the receiving space set, giving rise to a resulting wave at the receiving plane that progressively resolves the target profile  $|\Phi_T|^2$ . For  $Q = 0.95k$ , the entire target profile falls onto the range of well-coupled modes and the target profile  $|\Phi_T|^2$  is fully resolved. Looking at the required source profile  $|\Psi_T|^2$ , the incorporation of the phase front  $\exp(iQz_r)$  has the effect of shifting  $|\Psi_T|^2$  away from the  $y_s = 0$  line. In view of that, the parameter  $Q$  can be associated with a cone angle  $\theta$  that the wave vector of the propagating wave from the source to the receiving space makes with the optical axis, such that  $Q = \cos(\theta)k$ . From this association, we can relate  $Q$  with the position along the  $y_s$  axis,  $y_s = \pm Y_T$ , around which the required source profile  $|\Psi_T|^2$  is localized. Assuming a ray that travels from the point  $(x_s, y_s) = (0, Y_T)$  at the source plane to the center of the receiving horizontal plane  $(x_r, z_r) = (0, Z_r/2)$  with an angle  $\theta$  with respect to the optical axis, it can be shown that  $Y_T = (L + Z_r/2) \tan[\cos^{-1}(Q/k)]$ . For  $Q = 0.975k$  [Fig. S9 (b)] and for  $Q = 0.95k$  [Fig. S9 (c)], this expression yields, respectively,  $Y_T = 36.46\lambda$  and  $Y_T = 52.59\lambda$ , which is in accordance with the vertical positions occupied by  $|\Psi_T|^2$  in Figs S9(b-c).

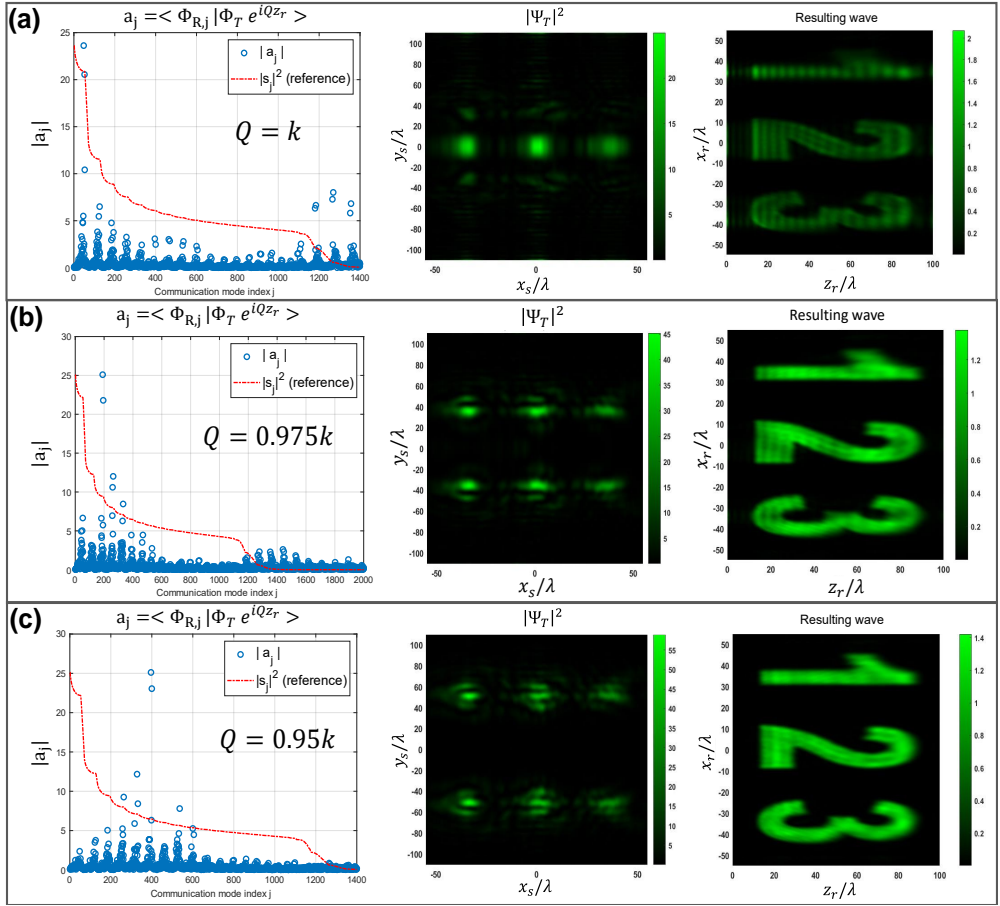

**Fig. S9.** Incorporating a plane wave phase front to project the entire target profile onto the range of well coupled modes. Simulation example assuming the source and receiving space configuration of Fig. 1(a), parameterized as listed on Table 1 and the target profile  $\Phi_T$  of Fig. 2(b). We apply a phase front of the form  $\exp(iQz_r)$ , with  $0 \leq Q \leq k = 2\pi/\lambda$ , to project the target profile onto the receiving space set. Examples shown for (a)  $Q = k$ , (b)  $Q = 0.975k$  and (c)  $Q = 0.95k$ . For each sub-figure, from left to right: amplitude of the inner product coefficients between  $\Phi_T \exp(iQz_r)$  and the receiving eigenfunctions  $\{\Phi_{R,j}\}$  (blue circles) and the coupling strengths  $|s_j|^2$  of the communication modes (in red dashed line, in arbitrary units); corresponding required source function intensity profile at the source plane and its resulting wave in the receiving horizontal plane, computed using the first 1200 modes.

## 7. SUPPLEMENTARY NOTE 7: SVD COMPUTATION TIME AND MEMORY STORAGE

Computation time and memory storage of the communication modes and their coupling strengths is analyzed in Fig. S10(a) for different scaling factor values  $\alpha$  applied to the source and receiving space configuration of Fig. 2(a) in the main text, parametrized as listed in Table 1. The arrays of source and receiving points and the separation distance  $L$  are multiplied by  $\alpha$  while the spacing distances in both spaces remain unchanged ( $\lambda$ ) to satisfy the criterion on the maximum allowed value for these distances (as described in Supplementary Note 3). The computation time was evaluated as the total time to compute the first  $M = 1.42N_{x,\text{str}}N_z$  communication modes in which  $N_{x,\text{str}}$  and  $N_z$  are evaluated from Eqs (S18) and (S19) in Supplementary Note 4<sup>2</sup>. We used a dedicated Server with processor Intel(R) Xeon(R) CPU ES-2690 0 @ 2.90 GHz. While for  $\alpha = 0.5$  the computation time is about 2 minutes, this time grows to almost 105 minutes for  $\alpha = 1$ . From that, scaling by only  $\alpha = 1.1$ , the computation time is 2.19 times larger, almost 230 minutes; and scaling by  $\alpha = 1.2$ , it is almost 329 minutes (3.1 times larger). In terms of memory storage, for  $\alpha = 1$  the communication modes and their coupling strengths require a total of about 516 MBytes. This number is significantly increased for  $\alpha = 1.2$ , reaching about 1.1 GBytes (almost two times larger). Both computation time and memory storage grow quite rapidly not only due to the increase in the size of the coupling matrix  $g_{ij}$  ( $N_R \times N_S$ ), which grows exponentially with  $\alpha$ , but also due to the increase in the number of well-coupled modes. This is illustrated in Fig. S10(b) which depicts the coupling strengths in order of decreasing size of their magnitude for different values of  $\alpha$ . On the right, the number of steps  $N_z$  and the number of strong effective modes of each step  $N_{x,\text{str}}$  present a roughly linear relationship with  $\alpha$ . Finally, to match the SLM effective display area, a scaling factor of  $\alpha = 40.5$  must be applied, which implies a number of about  $6.76 \times 10^{14}$  elements for the coupling matrix  $g_{ij}$ . Additionally, the coupling strength curve will present  $N_z = 756$  steps and each step will contain  $N_{x,\text{str}} = 2141$  effective strong modes. Thus, the SVD computation must be performed for the first  $M = 1618596$  well-coupled modes. Given the large magnitude of these numbers, an extremely huge computation time and memory storage must be dedicated to this case, which becomes highly unfeasible. Fitting the data of Fig. S10(a) by a polynomial function of third degree, a memory storage of 132.5 TBytes is estimated for  $\alpha = 40.5$ .

For the source and receiving space distribution of Fig. 2(b) in the main text and parametrized as listed in Table 1, i.e., the one containing a set of 10 receiving horizontal planes, the SVD computation time for the first  $M = 4000$  well-coupled modes is about 712 minutes and the memory storage is about 3.09 GBytes. For the distribution of Fig. 2(c) in the main text parametrized as listed in Table 1, this time is about 166 minutes for the first  $M = 1000$  well-coupled modes with a memory storage of about 657 MBytes. Scaling up these distributions to match the SLM effective display area will become even more critical in terms of computation time and memory storage.

<sup>2</sup>This expression for  $M$  can be split up in two terms:  $M = N_{x,\text{str}}N_z + 0.42N_{x,\text{str}}N_z$ . The first term is the total number of strong effective modes as analyzed in Supplementary Note 4. The factor  $0.42 N_{x,\text{str}}$  gives us the number of partially coupled modes of the first step as can be verified for the configuration of Fig. 2(a) in the main text parametrized as listed in Table 1 in Fig. S3(a). Thus, the second term estimates the total number of partially coupled modes. Notice that this last term is an overestimation, as the number of partially coupled modes within each step tends to decrease as we move towards higher steps.

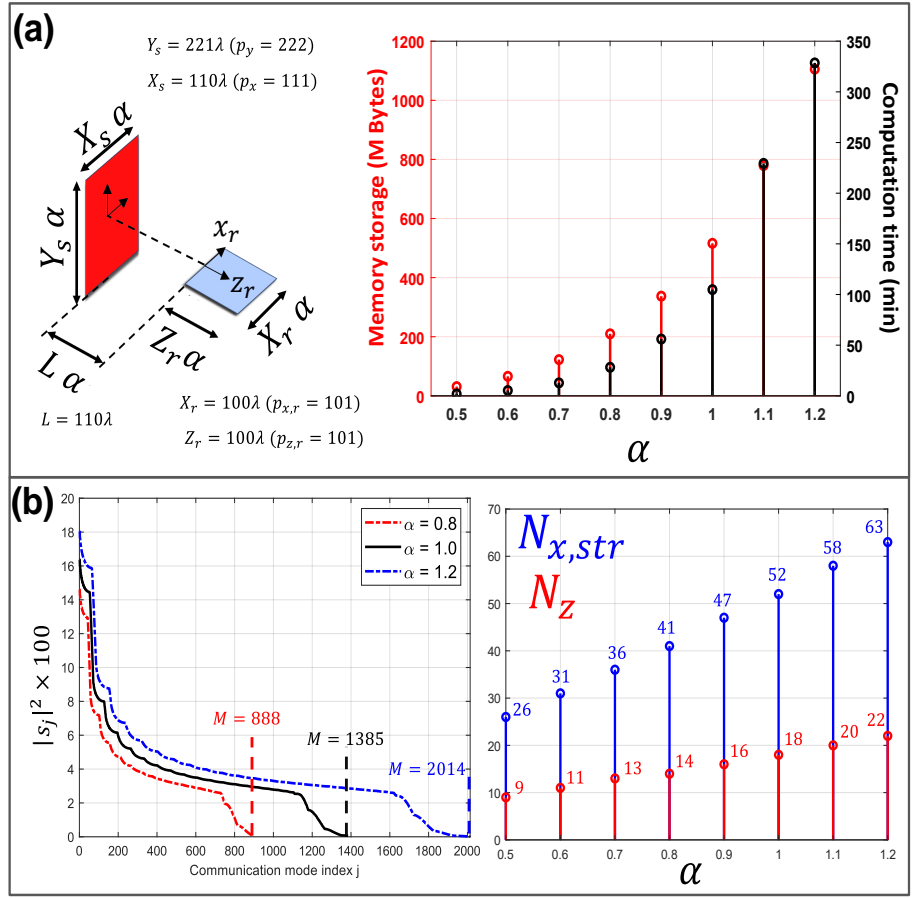

**Fig. S10. SVD computation time and memory storage** (a) Computation time (in black) and memory storage (in red) of the communication modes associated with the source and receiving space configuration of Fig. 2(a) in the main text and parametrized as listed in Table 1 is analyzed for a scaling factor  $\alpha$  applied to the arrays of source and receiving points and to the separation distance  $L$ . (b) On the left: coupling strengths in order of decreasing size of their magnitude for different values of  $\alpha$ . On the right: number of steps  $N_z$  (in red) and number of strong effective modes of each step  $N_{x, \text{str}}$  (in blue) for different values of  $\alpha$ .

## 8. SUPPLEMENTARY NOTE 8: ASPECT RATIO OF OUR RECONSTRUCTED STRUCTURED LIGHT WAVES USING OUR SLM OPTICAL SETUP

The wave solutions, computed as the resulting wave at the plane  $z_s = L$ , i.e.,  $\phi(x_s, y_s, L)$  from Eq. (4) in the main text, were scaled up to match the SLM effective display area. This leads to a magnification in the SLM of  $M_{\text{SLM}} = Y_{\text{SLM}}/Y_s$ , in which  $Y_{\text{SLM}} = 9000\lambda$  is the vertical dimension of the SLM effective display area. Additionally, our  $4f$  system [see Fig. 3(f) in the main text] alters the SLM out-going beam by a de-magnification of  $M_{4f} = f_2/f_1 = 3/4$ . Therefore, the resulting wave is magnified by a factor of  $M_{\text{SLM}}M_{4f}$  along its transverse dimensions. Its longitudinal dimension, on the other hand, is magnified by a factor of  $(M_{\text{SLM}}M_{4f})^2$ . For further details, see Ref. [6]. Therefore, the waves solutions computed from the source and receiving space configuration of Fig. 2(a) in the main text and parametrized as listed in Table 1 ( $Y_s = 221\lambda$ ), the transverse dimensions are scaled by  $\times M_{\text{SLM}}M_{4f} = (40.7)(3/4) = \times 30.5$  while the longitudinal dimension is stretched by a factor of  $\times (M_{\text{SLM}}M_{4f})^2 = \times 931.8$ . As a result, the aspect ratio of their reconstructed light waves is 1 : 30.5. Similarly, for the configuration of Fig. 2(b) parametrized as listed in Table 1 ( $Y_s = 150\lambda$ ), the spacing between the horizontal planes and their transverse dimension are scaled by a factor of  $\times 45$  while their longitudinal dimension by  $\times 2025$ .

The aspect ratio of our reconstructed light waves can be modified by altering the de-magnification ratio of the  $4f$  system in our optical setup [see Fig. 3(f) in the main text]. To achieve an aspect ratio of 1:1, we need to satisfy the condition  $M_{4f}M_{\text{SLM}} = 1$ , which implies  $f_1/f_2 = M_{\text{SLM}}$ . For the source and receiving space configuration of Fig. 2(a) in the main text, this could be implemented with  $f_1 = 400$  mm and  $f_2 = 10$  mm, resulting in a reconstructed light wave with the same dimensions as the simulated one, i.e.,  $X_r \times Z_r = 100\lambda \times 100\lambda$ . Notice that, however, since this light wave only extends longitudinally for a distance of  $53.2 \mu\text{m}$ , a more sophisticated optical setup than our currently one must be employed to properly measure a series of transverse planes of this light wave (i.e., to optically reconstruct it). This new system must include an objective lens and a motorized translational stage with a minimum repeatedly incremental motion as low as  $0.5 \mu\text{m}$ . Thus, to facilitate the reproducibility of our results through a simple optical setup albeit on the expense of distorting the aspect ratio of the light waves, we chose  $f_1 = 400$  mm and  $f_2 = 300$  mm for the  $4f$  system. This choice was also made to facilitate the comparison of our method with the light sheet wavefront shaping technique (see Supplementary Note 11) whose light waves extend over a longitudinal direction of tens of centimeters due to the use of Bessel beams with small cone angles [7].

## 9. SUPPLEMENTARY NOTE 9: PHASE RETRIEVAL ALGORITHM

Phase retrieval refers to a process of reconstructing a complex field by means of a phase-only platform. This process does not have a unique solution as the complex field can be encoded into a phase profile by many different approaches [8, 9]. In this paper, we followed the approach developed in Ref. [10].

First we normalize the complex field of the resulting wave at the  $z = L$  transverse plane  $\phi(x_s, y_s, L)$  and write it in terms of an amplitude  $a(x_s, y_s)$  term, ranging from  $[-1, 1]$ , and a phase profile term  $b(x_s, y_s)$ , ranging from  $[-\pi, \pi]$ , as:

$$\phi_n(x_s, y_s, L) = a(x_s, y_s) \exp[i b(x_s, y_s)], \quad (\text{S26})$$

in which the sub-index  $n$  refers to the normalized complex field.

Next, we need to convert  $\phi_n(x_s, y_s, L)$  into a phase transmittance mask of the form:

$$h(x_s, y_s) = \exp[i\Phi(a, b)], \quad (\text{S27})$$

in which we omit the explicit dependence on the spatial coordinates  $(x_s, y_s)$  of the functions  $a$  and  $b$ , and  $\Phi$  is a phase modulation function. Our goal now is to establish a function  $\Phi$  that properly encodes the complex field  $\phi_n$ , incorporating amplitude variations as phase variations. To do this, we expand  $h(x_s, y_s)$  into a Fourier series in the domain of the phase profile  $b$  as follows:

$$h(x_s, y_s) = \sum_{q=-\infty}^{\infty} c_q^a \exp(iqb), \quad (\text{S28})$$

where the coefficients  $c_q^a$ , which depend on the amplitude profile  $a$ , are given by:

$$c_q^a = \frac{1}{2\pi} \int_{-\pi}^{\pi} \exp[i\Phi(a, b)] \exp(-iqb) db. \quad (\text{S29})$$

Notice from Eqs S28 and S29 that the complex field  $\phi_n(x_s, y_s, L)$  is fully recovered from the first order term ( $q = 1$ ) if we satisfy the following condition, usually referred as the encoding condition:

$$c_1^a = Aa, \quad (\text{S30})$$

for a given positive constant  $A$ . Based upon this condition, sufficient and necessary conditions for the function  $\Phi(a, b)$  can be obtained, resulting in:

$$\int_{-\pi}^{\pi} \sin[\Phi(a, b) - b] db = 0, \quad (\text{S31a})$$

$$\int_{-\pi}^{\pi} \cos[\Phi(a, b) - b] db = 2\pi Aa, \quad (\text{S31b})$$

which implies that the phase modulation function  $\Phi(a, b)$  must present an odd symmetry in the variable  $b$ . In this paper, we adopted the following  $\Phi$  function:

$$\Phi(a, b) = f(a) \sin(b), \quad (\text{S32})$$

that corresponds to the phase mask of type 3 proposed in Ref. [10]. The factor  $f(a)$  in Eq. (S32) is obtained numerically from the encoding condition of Eq. (S30). Specifically, the corresponding Fourier coefficients for this phase modulation function, computed from Eq. (S29), are given by  $c_q^a = J_q[f(a)]$ , leading to the following encoding condition:

$$J_1[f(a)] = Aa. \quad (\text{S33})$$

We implemented a lookup table to numerically perform the Bessel function inversion in Eq. (S33). Choosing  $A = \max[J_1(\cdot)] = 0.5819$  leads to a function  $f(a)$  that acquires values over the interval  $0 \leq f(a) \leq 1.84$ . As a consequence, the phase domain of our phase mask  $h(x_s, y_s)$  is defined over the interval  $[-0.586\pi, 0.586\pi]$ , resulting in a total phase range of  $1.17\pi$ . For this phase range, our employed SLM can operate with a quantization of 800 gray levels.

Finally, we add a blazed grading with carrier spatial frequencies  $G_x$  and  $G_y$  to Eq. (S32). Thus, the phase mask that we encode onto the SLM is described by:

$$\Phi(a, b) = f(a) \sin[b + 2\pi(G_x x + G_y y)]. \quad (\text{S34})$$

## 10. SUPPLEMENTARY NOTE 10: PROJECTING AN ELLIPSOID

Here we consider another target 3D light distribution to be projected onto the eight inner horizontal receiving planes of the distribution shown in Fig. 1(c). Specifically, we project eight layers of an ellipsoid, centered in the middle of the receiving volume  $(x_r, y_r, z_r) = (0, 0, Z_r/2)$  and whose semiaxes have lengths  $a = 0.4X_r = 20\lambda$ ,  $b = 0.4Y_r = 54\lambda$  and  $c = 0.4Z_r = 20\lambda$ . The intensity of the target receiving profile  $|\Phi_T|^2$  and of the required source function  $|\Psi_T|^2$  are shown in Fig. S11(a). The optical reconstruction and its transverse planes at  $z_r = Z_r/2$  and at  $z_r = Z_r/4$  are shown in Fig. S11(b) while in Fig. S11(c) we present measured and simulated results of the four bottom layers. Notice that we have a good reconstruction for all the layers except the last one (layer 8) in which the resulting wave is not able to structure a circle nor to achieve the same intensity as the other layers. The reason for this is because the target circle we assigned to this layer has a diameter smaller than the characteristic minimum spot  $\Delta z$  our source transverse plane is capable of resolving (see Supplementary Note 5). To fully resolve the circle of this layer, we need to consider a source plane with a larger dimension along the  $y_s$  axis (large  $Y_s$  value and potentially with smaller spacing distances  $d_x$  and  $d_y$  for the additional source points), allowing us to incorporate a phase front  $\exp(iQz_r)$  with a smaller value of  $Q$ , resulting in a source function with a higher extent  $\Delta Y$  along the  $y_s$  axis, thus leading to a smaller value for  $\Delta z$ .

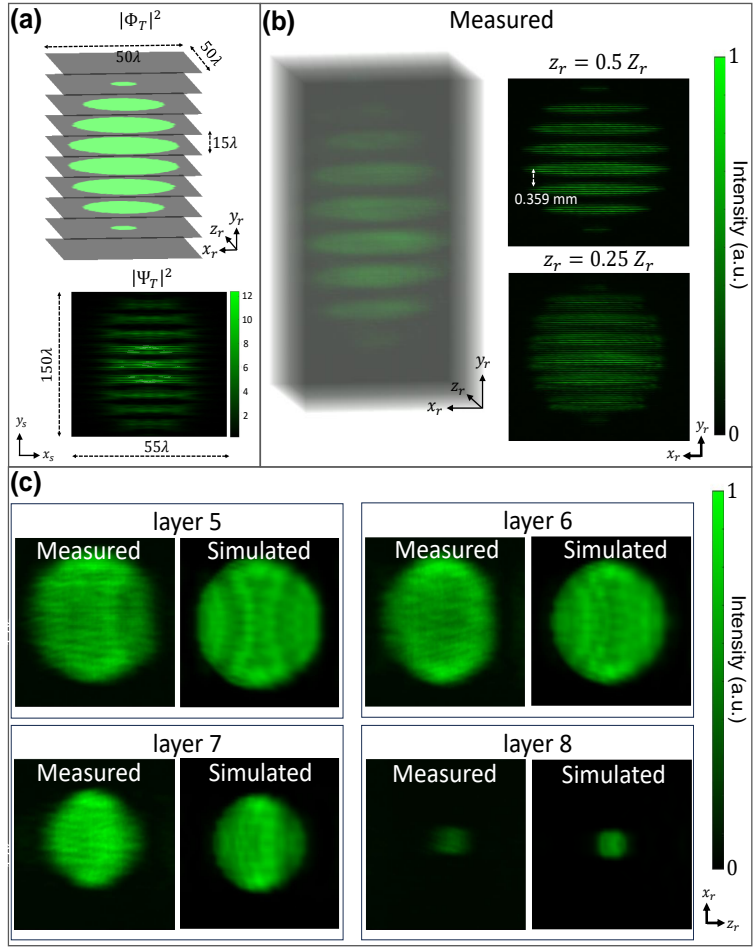

**Fig. S11. Projecting eight layers of an ellipsoid.** (a) An ellipsoid with dimensions  $20\lambda \times 54\lambda \times 20\lambda$  is projected over the eight inner horizontal receiving planes of the source-receiving space system of Fig. 1(c), parameterized as listed on Table 1. The resulting wave is computed using the first 3500 modes. (a) Target receiving intensity profile  $|\Phi_T|^2$  and its corresponding required source function intensity profile  $|\Psi_T|^2$ . (b) Optical reconstruction of the resulting wave using a phase-only SLM within a volume containing the receiving horizontal planes and at transverse planes located at the mid and quarter longitudinal distances,  $z_r = Z_r/2$  and  $z_r = Z_r/4$  ( $Z_r$ : longitudinal length of the planes). (c) Measured and simulated results for the four bottom ellipsoid layers. The wave solution is scaled up to match the SLM effective display area and thus the 1:1 aspect ratio of the simulated wave is not preserved in the measured results. Measured spacing distance between the horizontal planes is  $d_{y,r} = 0.359$  mm while their dimensions are  $Z_r \times X_r = 54$  mm  $\times$  1.20 mm.

## 11. SUPPLEMENTARY NOTE 11: CROSS-TALK AND COMPARISON WITH LIGHT SHEET METHOD

To evaluate the level of cross-talk at each horizontal plane  $i$  that compose the receiving space of the example in Fig. 5 in the main text, we use the following figure of merit:

$$\epsilon_i = \frac{\iint_{S_i} ||\phi_n(\mathbf{r}_{S_i})|^2| - |\phi_{n,\text{ref}}(\mathbf{r}_{S_i})|^2| dS_i}{\iint_{S_i} (|\phi_n(\mathbf{r}_{S_i})|^2| + |\phi_{n,\text{ref}}(\mathbf{r}_{S_i})|^2) dS_i}, \quad (\text{S35})$$

in which  $\phi_n$  refers to the normalized resulting wave computed from Eq. (4) in the main text,  $S_i$  is the surface of the horizontal plane  $i$ ,  $\mathbf{r}_{S_i}$  is a vector position that describes  $S_i$  and  $\phi_{n,\text{ref}}$  is the normalized resulting wave when only the target intensity profile in the horizontal plane  $i$  is projected, i.e., in all other planes the target intensity profile is set to zero. Thus,  $\epsilon_i = 0$  means that  $\phi_n(\mathbf{r}_{S_i})$  is perfectly identical to  $\phi_{n,\text{ref}}(\mathbf{r}_{S_i})$  in amplitude and therefore the projection of the target intensity profile in the plane  $i$  is done without cross-talk. In Fig. S12(a), we show the intensity of both  $\phi_{n,\text{ref}}(\mathbf{r}_{S_i})$  and  $\phi_n(\mathbf{r}_{S_i})$  for all eight horizontal planes of the example of Fig. 5 in the main text. The level of cross-talk, evaluated from Eq. (S35), in each plane is also shown. Notice that  $\epsilon$  assumes a value lower than 0.1 in all eight planes, indicating, in fact, the low level of crosstalk between the reconstructed intensity profiles.

Projecting the same target intensity profiles using the light sheet wavefront shaping method is analyzed in Fig. S12(b). Similarly as in Ref. [7], to compose each light sheet, we employed light threads with spot size radius of  $r_0 = 30\mu\text{m}$  and a gap of  $45\mu\text{m}$  between them. To match the size of the reconstructed horizontal planes obtained from our method using our SLM optical setup,  $Z_r \times X_r = 54\text{ mm} \times 1.20\text{ mm}$ , each light thread extends for a longitudinal distance of  $L = 54\text{ cm}$  and each light sheet is composed of  $P = 28$  light threads. We used a total of  $2N + 1 = 95$  Bessel modes to modulate each light thread. The spacing between the light sheets is the same spacing distance between our reconstructed horizontal planes,  $0.359\text{ mm}$  (i.e.,  $11.97 r_0$ ). Finally, the resulting wave is computed by adding all the superposition of Bessel modes (see details in Ref. [7]). The intensity of the reference and normalized resulting waves in all eight horizontal planes and the cross-talk of each plane are shown in Fig. S12(b). In contrast to our method, notice that here the projection in all the planes is highly affected by cross-talk, greatly distorting the intensity profiles of the digits.

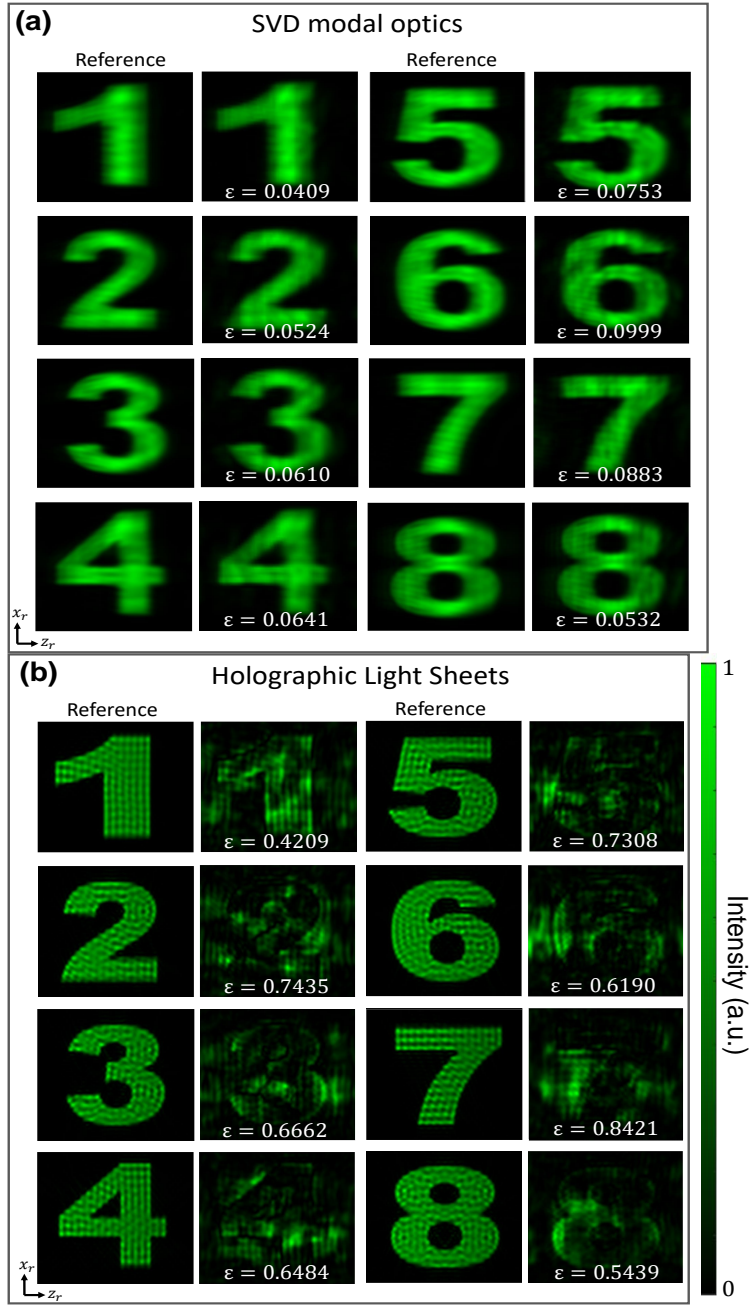

**Fig. S12. Comparing SVD modal optics and holographic light sheet approaches** For the example shown in Fig. 5 in the main text, we compare the reconstructed intensity profiles in all the eight horizontal planes using (a) wavefront shaping method based on communication modes and (b) the Light Sheet wavefront shaping method. The columns labeled ‘Reference’ present the intensity of the resulting wave when only the target intensity profile assigned to that particular plane is projected. We evaluate the level of cross-talk  $\epsilon$  in each plane by comparing the intensity of the resulting wave in that plane with its reference wave according to Eq. (S35). A value of  $\epsilon = 0$  means that the resulting wave is perfectly identical to its reference wave in amplitude and thus the projection is done without cross-talk.

## 12. SUPPLEMENTARY NOTE 12: REDUCING THE SEPARATION DISTANCE BETWEEN THE HORIZONTAL RECEIVING PLANES

We apply the same target intensity profile of the example of Fig. 5 in the main text. The only difference is that the spacing distance between the horizontal receiving planes are reduced to  $d_{y,r} = 10\lambda$  [Fig. S13(a)] and to  $d_{y,r} = 7.5\lambda$  [Fig. S13(b)]. The resulting wave is computed using the first 3500 well-coupled modes and the cross-talk in each plane is evaluated from Eq. (S35).

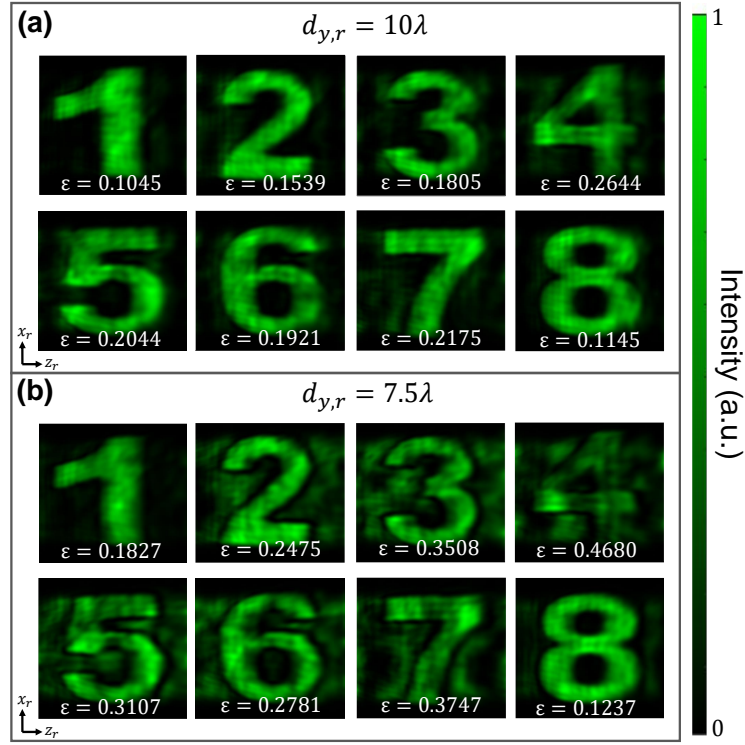

**Fig. S13. Reducing the spacing distance between the receiving horizontal planes.** We consider the source-receiving space system of Fig. 1(c) in the main text parameterized accordingly to Table 1 except that the spacing between the horizontal receiving planes is reduced to (a)  $d_{y,r} = 10\lambda$  and to (b)  $d_{y,r} = 7.5\lambda$ . These spacing distances correspond to 0.2394 mm and 0.179 mm when the corresponding wave solutions are encoded in our SLM optical setup. Similarly to the example of Fig. 5 in the main text, we project eight digits in the eight inner horizontal receiving planes, modulate the target profile with a phase front  $\exp(iQz_r)$  with  $Q = 0.95k$  and compute the resulting wave using the first 3500 modes.

### 13. SUPPLEMENTARY NOTE 13: PROJECTING STRUCTURED LIGHT WAVES ON THE LONGITUDINAL SURFACE OF A CYLINDER

In this example, the target profile consists of the target 2D image of Fig. 2(b) projected onto the longitudinal cylindrical surface of the source-receiving system of Fig. 1(d), parameterized accordingly to Table 1. We modulate this target profile  $\Phi_T$  with a phase front  $\exp(iQz_r)$  with  $Q = 0.95k$  and compute its corresponding source function  $\Psi_T$  using the first 800 well-coupled modes. Fig S14(a) shows the intensity of both the target and the required source function. The simulated and reconstructed (measured) resulting waves are shown in Figs S14(b) and (c), from left to right, within a volume containing the receiving space, on the longitudinal surface of the cylinder as a function of the azimuth angle  $\phi_r = \text{atan}(y_r/x_r)$  and the longitudinal distance  $z_r$ , and at the mid-transverse plane of the cylinder ( $z_r = Z_r/2$ ). The measured dimensions are indicated in red in Fig. S14(c). Notice that our wavefront shaping method based on communication modes, in addition to providing a reconstructed profile with high intensity uniformity and contrast within the receiving curved surface, leads to a light wave with dark intensity along the optical axis over the entire longitudinal distance of the cylinder. When reducing the radius of the cylinder surface by half, although the target intensity profile is still well reconstructed on the cylindrical surface, it comes at the expense of introducing a high intensity inside the cylinder, as shown in Fig. S14(d). This intensity reaches a value that is almost 11 times higher than the intensity on the surface, as depicted in Fig. S14(e).

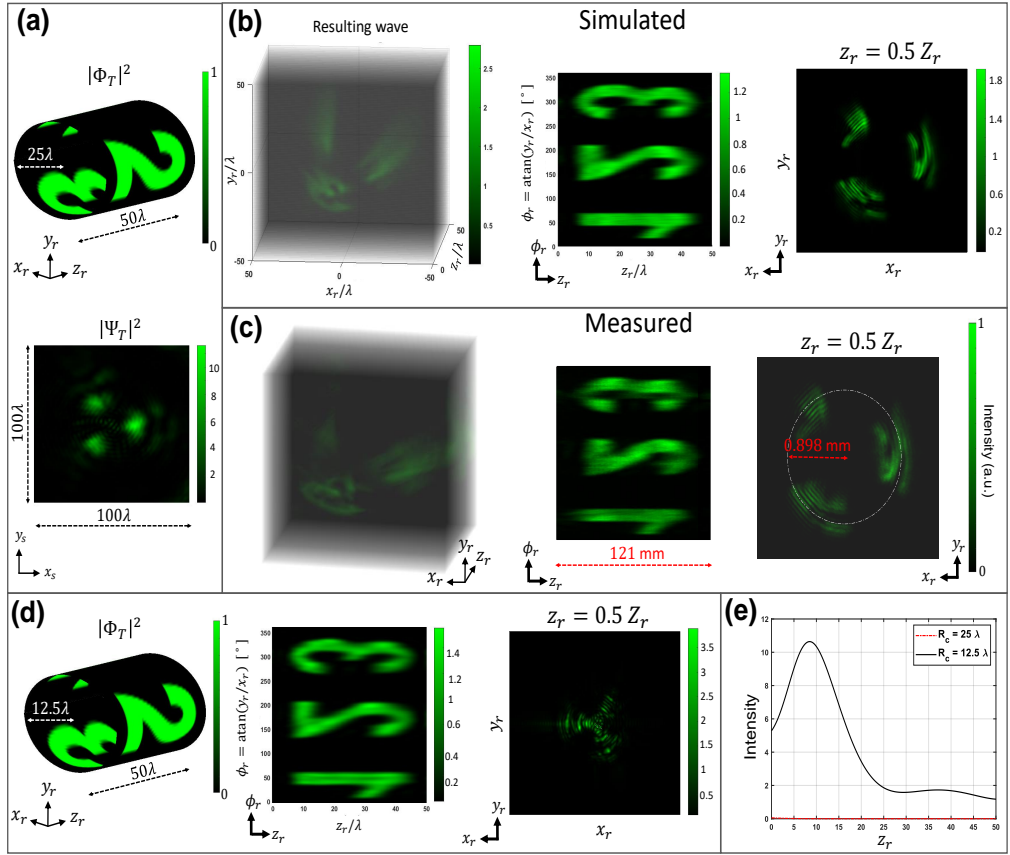

**Fig. S14. Structured light field over the longitudinal surface of a cylinder using communication modes**  
The source and receiving configuration is the one shown in Fig. 1(d) in the main text, parameterized as listed on Table 1. (a) Target intensity distribution  $|\Phi_T|^2$  consists of the grayscale amplitude profile of 2D image of Fig. 2(b) projected onto the receiving cylindrical surface. Its required source function  $|\Psi_T|^2$  is computed using the first 800 well-coupled modes. (b) From left to right: simulated resulting wave over a volume containing the receiving space, over the lateral cylindrical surface (described in terms of its azimuth angle and the longitudinal coordinate  $z_r$ ) and at the mid transverse plane of the receiving space. (c) Optical reconstruction of the resulting wave using a phase-only SLM. Measured dimensions: longitudinal distance  $Z_r = 121$  mm and radius  $R_r = 0.898$  mm. (d) Resulting wave when the radius of the cylindrical surface is reduced by half (from  $25\lambda$  to  $12.5\lambda$ ). (e) Intensity inside the cylinder along the optical axis.

## REFERENCES

1. D. A. B. Miller, "Waves, modes, communications, and optics: a tutorial," *Adv. Opt. Photon.* **11**, 679–825 (2019).
2. D. A. B. Miller, "Spatial channels for communicating with waves between volumes," *Opt. Lett.* **23**, 1645–1647 (1998).
3. D. A. B. Miller, "An introduction to functional analysis for science and engineering," (2019). <https://arxiv.org/abs/1904.02539>.
4. D. Porter and D. Stirling, *Integral Equations: A Practical Treatment, from Spectral Theory to Applications*, Cambridge Texts in Applied Mathematics (Cambridge University Press, 1990).
5. D. A. B. Miller, Z. Kuang, and O. D. Miller, "Tunnelling escape of waves," *Nat. Photonics* (2024). Published online, Dec. 3, 2024, <https://www.nature.com/articles/s41566-024-01578-w>.
6. M. Zamboni-Rached, G. d. A. Lourenço-Vittorino, T. Viana de Sousa *et al.*, "Mathematical description of a Frozen Wave beam after passing through a pair of convex lenses with different focal distance," *arXiv e-prints arXiv:1907.08202* (2019).
7. A. H. Dorrah, M. Zamboni-Rached, and M. Mojahedi, "Wavelength and topological charge management along the axis of propagation of multichromatic non-diffracting beams," *J. Opt. Soc. Am. B* **36**, 1867–1872 (2019).
8. A. Forbes, A. Dudley, and M. McLaren, "Creation and detection of optical modes with spatial light modulators," *Adv. Opt. Photon.* **8**, 200–227 (2016).
9. C. Rosales-Guzmán, A. Forbes, and S. of Photo-Optical Instrumentation Engineers, *How to Shape Light with Spatial Light Modulators*, SPIE. Spotlight (SPIE Press, 2017).
10. V. Arrizón, U. Ruiz, R. Carrada, and L. A. González, "Pixelated phase computer holograms for the accurate encoding of scalar complex fields," *J. Opt. Soc. Am. A* **24**, 3500–3507 (2007).
